# Supplementary material for: Column Selection via Adaptive Sampling
Source: arXiv:1510.04149 source file (2015-10-14)
Supplement: Supplementary file 1 [file appendix.tex]

\section{Appendix XXX STILL NEEDS WORK XXX}

\subsection{Algorithm and Proof of  Eqn 1}
We can write $(\matC \matC^+ \matA)_k = \matC \matX,$ ($\matX$ has rank at most $k$) \cite{BMD11} where
\begin{equation}
 \matX = \argmin_{\matPsi \in \mathbb{R}^{c \times n}:rank(\matPsi)\leq k} \FNormS{\matA -\matC\matPsi}. \nonumber
\end{equation}%\vskip -0.2cm
This can be achieved by the following algorithm (Lemma 8 of \cite{BMD11}).\\
1. Orthonormalize the columns of $\matC$ in $O(mc^2)$ time to construct the matrix $\matQ \in \mathbb{R}^{m\times c}.$\\
2. Compute $(\matQ^T\matA)_k \in \mathbb{R}^{c\times n}$ via SVD in $O(mnc+nc^2).$\\
3. Return $\matQ(\matQ^T\matA)_k \in \mathbb{R}^{m\times n}$ in $O(mnk)$ time. \\
Since $\matQ$ is an orthonormal basis for the column space of $\matC,$ $(\matC \matC^+ \matA)_k = (\matQ \matQ^+ \matA)_k.$  Thus,
$$\FNormS{\matA-(\matC\matC^+\matA)_k}=\FNorm{\matA-(\matQ\matQ^+\matA)_k} = \min_{\matPsi:rank(\matPsi)\leq k} \FNormS{\matA -\matQ\matPsi}$$
Using matrix-Pythagoras and orthonormality of $\matQ,$
$$\FNormS{\matA -\matQ\matPsi} =\FNormS{\matA -\matQ\matQ^T\matA + \matQ(\matQ^T\matA- \matPsi)} = \FNormS{\matA -\matQ\matQ^T\matA}+\FNormS{\matQ^T\matA- \matPsi}.$$
Setting $\matPsi = (\matQ^T\matA)_k$ minimizes the above quantity over all rank-k matrices $\matPsi.$

\subsection{Column Selection Algorithms}
In this Section, we describe the two column-selection algorithms used with the adaptive sampling algorithm.

\subsubsection{Near Optimal column Selection}\label{subsec:dsf}
Near optimal column-selection \cite{BMD11} consists of random projections, followed by two rounds of column sampling, with the first round of sampling done with the deterministic Dual-set Spectral Frobenius Sparsification and a second round of randomized sampling with an additive-error column selection algorithm from the residual of the first round. The random projection step was used to improve running time. Since running time is not a concern for us, we perform the two-step column sampling directly using Dual-set Spectral Frobenius Sparsification and a second round of randomized sampling with an additive-error column selection algorithm from the residual of the first round. The algorithm is stated as Algorithm~\ref{alg:alg_dsf2}. Next, we state the main result of near-optimal column-selection from \cite{BMD11} in terms of expectation as Lemma~\ref{lem:dsf_ran2} and then show how we can get a high probability result.

\begin{lemma}
(Column Selection by Dual-Set Spectral Frobenius Sparsification and additive-error sampling)\cite{BMD11}.Given a matrix $\matA \in \mathbb{R}^{m\times n}$ of rank $\rho,$ a target rank $k<\rho,$ and $0<\epsilon<1,$ there exists a randomized algorithm to select at most $c=\frac{2k}{\epsilon}(1+o(1))$ columns of $\matA$ and form a matrix $\matC \in \mathbb{R}^{m\times c}$ such that
$$\Expect{\FNormS{\matA-(\matC\matC^+\matA)_k}}\leq (1+\epsilon) \FNormS{\matA-\matA_k}.$$
The algorithm runs in $O\left(mn\min\{m,n\}+nrk^2+mn+ n\log(1/\epsilon) \right)$ time.
\label{lem:dsf_ran2}
\end{lemma}

Notice that $(\matC\matC^+\matA)_k$ is a random variable. Then,
$$\Expect{\FNormS{\matA-(\matC\matC^+\matA)_k}-\FNormS{\matA-\matA_k}} \leq \epsilon\FNormS{\matA-\matA_k}.$$ The left hand side of the inequality is a random variable $\geq 0.$ This is because $\matA-\matA_k$ is the best rank-$k$ reconstruction error of $\matA$ and $\FNorm{\matA-(\matC\matC^+\matA)_k}$ will always be larger than $\FNorm{\matA-\matA_k}.$ Now, using Markov's inequality, with probability at least $1/2,$ $$\Expect{\FNormS{\matA-(\matC\matC^+\matA)_k}}\leq (1+2\epsilon) \FNormS{\matA-\matA_k}.$$
Repeat the second part of the algorithm multiple times and choose columns with the minimum error.  To reduce the failure probability to $\delta,$ we repeat the process $(1/2)^{\log_2(1/\delta)}$ times. We re-state the lemma in terms of high probability as Lemma~\ref{lem:dsf_ran}.

\begin{lemma}
(Column Selection by Dual-Set Spectral Frobenius Sparsification and additive-error sampling)\cite{BMD11}.Given a matrix $\matA \in \mathbb{R}^{m\times n}$ of rank $\rho,$ a target rank $k<\rho,$ and $0<\epsilon<1,$ there exists a randomized algorithm to select at most $c=\frac{2k}{\epsilon}(1+o(1))$ columns of $\matA$ and form a matrix $\matC \in \mathbb{R}^{m\times c}$ such that with probability $1-\delta$, for $0<\delta<1,$
$$\FNormS{\matA-\matC\matC^+\matA} \leq \FNormS{\matA-(\matC\matC^+\matA)_k} \leq (1+\epsilon) \FNormS{\matA-\matA_k}.$$
The algorithm runs in $O\left( mn \min\{m,n\}+nrk^2 + mn + n\log c \log(1/\delta) \right)$ time.
\label{lem:dsf_ran}
\end{lemma}

\begin{algorithm}[thb]
\begin{small}
\begin{framed}
\textbf{Input:}  $\matA \in \mathbb{R}^{m\times n},$ target rank $k,$ two integers $r$ and $s.$  \\
\textbf{Output:} Sampling matrix $\matS.$
\begin{enumerate}
\item $\matS_1 \leftarrow \text{Dual-Set Spectral Frobenius Sparsification}(\matV, \matA, r).$
\item Compute $\matC_1=\matA\matS.$ Then, compute $\matB = \matA -\matC_1 \matC_1^+\matA.$
\item Sample $s$ columns from $\matA$ in $s$ i.i.d trials with probability $p_i = \TNormS{\b_i}/\FNormS{\matB}$ for $i=1,\cdots,n$ and get $\matS_2.$
\item Compute $\matC_2 =\matA \matS_2.$
\item $\matS =[\matS_1, \matS_2].$
\item Return $\matS.$
\end{enumerate}
\end{framed}
\caption{Near-optimal column selection algorithm}
\label{alg:alg_dsf2}
\end{small}
\end{algorithm}

\subsubsection{Dual-set Spectral Frobenius Sparsification}
The Dual-set Spectral Frobenius Sparsification by Boutsidis et al \cite{BMD11} is a deterministic algorithm used for column-selection. Lemma~\ref{lem:dsf_det} is the result for column-selection by using dual-set Spectral-Frobenius sparsification. We state the main lemma of the algorithm as Lemma \ref{lem:lem_dsf} and the algorithm as Algorithm~\ref{alg:alg_dsf}.

\begin{lemma}
(Column Selection by Dual-Set Spectral Frobenius Sparsification)\cite{BMD11}. Given a matrix $\matA \in \mathbb{R}^{m\times n}$ of rank $\rho$ and a target rank $k<\rho,$ there exists a deterministic algorithm to select $r>k$ columns of $\matA$ and form a matrix $\matC \in \mathbb{R}^{n\times r}$ such that,
$$\FNormS{\matA-\matC\matC^+\matA} \leq \FNormS{\matA-(\matC\matC^+\matA)_k} \leq \left(1+\frac{1}{\left(1-\sqrt{k/r}\right)^2}\right) \FNormS{\matA-\matA_k}.$$
The algorithm runs in $O\left( mn \min\{m,n\}+nrk^2 \right)$ time.
\label{lem:dsf_det}
\end{lemma}

\begin{lemma} (Dual-Set Spectral Frobenius sparsification) \cite{BMD11}
Let $\mathcal{U}= \{\x_1,\cdots, \x_n \} \subset \mathbb{R}^\ell (\ell<n)$ contain the columns of an arbitrary matrix $\matX \in \mathbb{R}^{\ell \times n}.$ Let $\mathcal{V}=\{\v_1,\cdots,\v_n \} \subset \mathbb{R}^k (k<n)$ be a decomposition of the identity, that is $\sum_{i=1}^n \v_i \v_i^T =\matI_k.$ Given an integer $r$ with $k<r<n,$ Algorithm \ref{alg:alg_dsf} deterministically computes a set of weights $s_i \geq 0 \; (i=1,\cdots, n)$ at most $r$ of which is non-zero, such that
$$\lambda_k \left(\sum_{i=1}^n s_i \v_i \v_i^T \right) \geq \left(1-\sqrt{k/r}\right)^2, \;\; \text{and}\;\;  \bf{Tr}\left( \sum_{i=1}^n s_i \x_i \x_i^T\right) \leq \bf{Tr} \left(\sum_{i=1}^n \x_i \x_i^T \right).$$
Equivalently, if $\matV \in \mathbb{R}^{n\times k}$ is a matrix whose rows are the vectors $\v_i^T,$ $\matX\in \mathbb{R}^{n\times \ell}$ is a matrix whose rows are the vectors $\x_i^T,$ and $\matS \in \mathbb{R}^{n\times r}$ be the sampling matrix containing the weights $s_i>0$, then:
$$\sigma_k \left(\matV^T \matS \right) \geq 1- \sqrt{k/r}, \; \; \text{and} \;\; \FNormS{\matX^T \matS} \leq \FNormS{\matX}.$$ The weights $s_i$ can be computed deterministically in $O(rnk^2+n\ell)$ time.
\label{lem:lem_dsf}
\end{lemma}

\begin{algorithm}[thb]
\begin{small}
\begin{framed}
\textbf{Input:}  $\mathcal{U}= \{\x_i \}_{i=1}^n \subset \mathbb{R}^\ell (\ell<n); \mathcal{V}=\{\v_i\}_{i=1}^n \subset \mathbb{R}^k (k<n),$ with $\sum_{i=1}^n \v_i \v_i^T =\matI_k,$ $k<r<n.$  \\
\textbf{Output:} Sampling matrix $\matS.$
\begin{enumerate}
\item Initialize $\matS = \bf{0}_{d\times r}, \matB_0 = \bf{0}_{k\times k}.$
\item \textbf{for} $\tau = 0,\cdots, r-1$ \textbf{do}
\item $\;\;\;$ Set $L_\tau = \tau- \sqrt{rk}.$
\item $\;\;\;$ Pick index $i \in \{1,2,\cdots,n \}$ and $t$ such that $$\left(1-\sqrt{\frac{k}{r}}\right) \frac{\x_i^T \x_i}{\FNormS{\matX}} \leq \frac{1}{t} \leq \frac{\v_i^T \left(\matB_\tau -(L_\tau+1)\matI_k \right)^{-2} \v_i}{\phi(L_\tau+1, \matB_\tau) - \phi(L_\tau,\matB_\tau)} - \v_i^T\left(\matB_\tau - (L_\tau+1)\matI_k \right)^{-1}\v_i$$ $\;\;\;$where
$ \phi(L,\matB) = \sum_{i=1}^k \left( \lambda_i(\matB) -L \right)^{-1}.$
\item $\;\;\;$ Update $\matB_{\tau+1} = \matB_\tau + t\v_i\v_i^T.$ Set $\matS_{i\tau}=1.$
\item \textbf{end for}
\item Return $\matS.$
\end{enumerate}
\end{framed}
\caption{Dual Set Spectral Frobenius Sparsification Algorithm}
\label{alg:alg_dsf}
\end{small}
\end{algorithm}

\subsubsection{Leverage-score Sampling}\label{subsec:lvg_algo}
Our randomized feature selection method is based on importance sampling or the so-called leverage-score sampling of \cite{DrineasrelativeCUR}. Let $\matV$ be the top-$k$ right singular vectors of the data matrix $\matA \in \mathbb{R}^{m\times n}$. A carefully chosen probability distribution of the form
\vskip -0.4cm
\begin{equation}
p_i = \frac{\TNormS{\matV_{i}}}{n}, \text{ for } i=1,2,...,n,
\label{eqn:eqnlvg}
\end{equation}
i.e. proportional to the squared Euclidean norms of the rows of the right-singular vectors is constructed. Select $r$ rows of $\matV$ in i.i.d trials and re-scale the rows with $1/\sqrt{p_i}$. The time complexity is dominated by the time to compute the SVD of $\matA$.

\begin{lemma}
(Column Selection by Leverage-Score Sampling).\cite{DrineasrelativeCUR} Given a matrix $\matA \in \mathbb{R}^{m\times n}$ of rank $\rho,$ a target rank $k<\rho,$ and let $\epsilon \in (0,1].$ There exists a randomized algorithm to select $c=O(k\log(k/\epsilon^2))$ columns of $\matA$ and form a matrix $\matC \in \mathbb{R}^{n\times c}$ such that with probability at least 0.7,
$$\FNorm{\matA-\matC\matC^+\matA} \leq \FNorm{\matA-(\matC\matC^+\matA)_k} \leq (1+\epsilon) \FNorm{\matA-\matA_k}.$$
The algorithm runs in $O\left( mn \min \{m,n\}\right)$ time.
\label{lem:lvg}
\end{lemma}

\subsection{Experimental Results}
We compare adaptive sampling with sequential sampling of columns with near-optimal column selection, leverage-score sampling and additive-error column selection. The number of columns chosen in the $\ell$th iteration of sequential sampling is same as the number of columns selected in $\ell$ rounds by adaptive sampling. Fig \ref{fig:adp_vs_seq} shows the residuals for sequential vs adaptive sampling for the various methods and datasets for $r=2k.$ For AE and LVG, sequential and adaptive sampling are comparable, while for Nopt, adaptive sampling is better than sequential sampling in most cases. Though sequential sampling and adaptive sampling are comparable in practice, in theory, we show that it is possible to get a tighter bound with adaptive sampling. This seems to imply that the theoretical bounds for sequential sampling can be improved.

\noindent \textbf{Dataset.}Our second dataset consists of SNPs data of human chromosomes from the HGDP database \cite{Pasch10}. The features in this dataset correspond to Single Nucleotide Polymorphisms (SNPs), which are well-known biallelic loci of genetic variation across the human genome. Each entry in the resulting matrix is set to $+1$ (homozygotic in one allele), $-1$ (homozygotic in the other allele), or $0$ (heterozygotic), depending on the genotype of the respective SNP for a particular sample. Missing entries were filled in with $-1$, $+1$, or $0$, with probability 1/3.

\begin{figure}[!htb]
\begin{center}
\includegraphics[height = 45mm,width=\columnwidth,clip]{techtc_49_adp_vs_1pass_r2k.eps}
\includegraphics[height = 45mm,width=\columnwidth,clip]{hgdp_22_adp_vs_1pass_r2k.eps}
\includegraphics[height = 45mm,width=\columnwidth,clip]{synth_data1_1pass_vs_adp.eps}
\includegraphics[height = 45mm,width=\columnwidth,clip]{synth_data2_1pass_vs_adp.eps}
\end{center}
\caption{\small Sequential vs adaptive sampling for TechTC, HGDP and Synthetic datasets when $r=2k.$}
\label{fig:adp_vs_seq}
\end{figure}

\begin{figure}[!htb]
\begin{center}
\includegraphics[height = 50mm,width=\columnwidth,clip]{techtc_49docs_niter10_r1_5k.eps}
\includegraphics[height = 50mm,width=\columnwidth,clip]{techtc_49docs_niter10_r1_75k.eps}
\includegraphics[height = 50mm,width=\columnwidth,clip]{techtc_49docs_niter10_r4k.eps}
\end{center}
\caption{\small Plots of relative error ratio using various adaptive sampling algorithms averaged over 49 TechTC-300 datasets.}
\label{fig:plots_techtc}\vskip -0.6cm
\end{figure}

\begin{figure}[!htb]
\begin{center}
\includegraphics[height = 50mm,width=\columnwidth,clip]{hgdp_allchromo_niter10_r1_5k.eps}
\includegraphics[height = 50mm,width=\columnwidth,clip]{hgdp_allchromo_niter10_r1_75k.eps}
\includegraphics[height = 50mm,width=\columnwidth,clip]{hgdp_allchromo_niter10_r4k.eps}
\end{center}
\caption{\small Plots of relative error ratio using various adaptive sampling algorithms for HGDP dataset averaged over 22 chromosomes.}
\label{fig:plots_hgdp}\vskip -0.6cm
\end{figure}

\begin{figure}[!htb]
\begin{center}
\includegraphics[height = 50mm,width=\columnwidth,clip]{synth_data1_r1_5k.eps}
\includegraphics[height = 50mm,width=\columnwidth,clip]{synth_data1_r1_75k.eps}
\includegraphics[height = 50mm,width=\columnwidth,clip]{synth_data1_r4k.eps}
\end{center}
\caption{\small Plots of relative error ratio using various adaptive sampling algorithms for Synthetic Dataset 1.}
\label{fig:plots_techtc}\vskip -0.6cm
\end{figure}

\begin{figure}[!htb]
\begin{center}
\includegraphics[height = 50mm,width=\columnwidth,clip]{synth_data2_r1_5k.eps}
\includegraphics[height = 50mm,width=\columnwidth,clip]{synth_data2_r1_75k.eps}
\includegraphics[height = 50mm,width=\columnwidth,clip]{synth_data2_r4k.eps}
\end{center}
\caption{\small Plots of relative error ratio using various adaptive sampling algorithms for Synthetic Dataset 2.}
\label{fig:plots_techtc}\vskip -0.6cm
\end{figure}
